# Supplementary material for: DDTNet: Degradation Disentanglement and Transfer Network for Test-Time All-in-One De-weathering Adaptation
Source: arXiv:2606.16298 source file (2026-06-15)
Supplement: Supplementary file 1 [file X_suppl.tex]

\clearpage
\setcounter{page}{1}
\maketitlesupplementary

% ---- 附錄專用設定 ----
% 圖表編號從 A1, A2, ... 開始
\setcounter{figure}{0}
\setcounter{table}{0}

% 統一控制附錄大圖的寬度（覺得太大可改成 0.85 或 0.8）
\newcommand{\appfigwidth}{0.95\textwidth}

% \begin{figure*}[t]
%   \centering
%   \includegraphics[
%     width=\appfigwidth,
%     height=0.95\textheight,
%     keepaspectratio
%   ]{appendix_img/generate_data.pdf}
%   \vspace{-0.4em}
%   \caption{Pipeline of data synthesis and optimization in DDTNet. We synthesize degraded–clean triplets sharing the same degradation but different content, enabling end-to-end optimization of the network.}
%   \label{fig:Gen_data}
%   \vspace{-0.3em}
% \end{figure*}

% ====== 修改開始：將 figure* 改為 strip ======
% strip 環境會強制內容在當前位置跨雙欄顯示，不會浮動到下一頁
\begin{strip}
  \centering
  \includegraphics[
    width=\appfigwidth,
    height=0.5\textheight, % 建議稍微縮小一點高度，以免第一頁被撐爆導致文字很少
    keepaspectratio
  ]{appendix_img/generate_data.pdf}
  \vspace{-0.4em}
  % 注意：在非 figure 環境中，必須使用 \captionof{figure}{...}
  \captionof{figure}{Pipeline of data synthesis and optimization in DDTNet. We synthesize degraded–clean triplets sharing the same degradation but different content, enabling end-to-end optimization of the network.}
  \label{fig:Gen_data}
  \vspace{-0.3em}
\end{strip}

%---------------------------------------------------------------
\section{Pipeline of Data Synthesis and Optimization in DDTNet}
\label{sec:app:pipeline}
%---------------------------------------------------------------

As shown in Figure~\ref{fig:Gen_data}, we collect degraded–clean triplets that share the same degradation patterns but differ in content.
For rainy and snowy images, we use the degradation masks (rain streaks and snow masks) from Rain100H~\citep{Yang_2017_CVPR}, Rain100L~\citep{Yang_2017_CVPR}, and Snow100K~\citep{liu2018desnownet} to synthesize the degraded images.
For hazy images, we directly adopt the RESIDE dataset~\citep{li2019benchmarking}, which provides hazy images sharing the same haze characteristics (haze density and atmospheric light) but differing in content. 
Next, we describe the data synthesis process for generating rainy, snowy, and hazy images.

\paragraph{Rain and snow.}
Given a clean image $I^c \in \mathbb{R}^{H \times W \times 3}$, we utilize rain or snow masks
$M \in \mathbb{R}^{H \times W \times 1}$, $M \in [0,1]$, to generate a rainy or snowy image
$I^d \in \mathbb{R}^{H \times W \times 3}$ as
\begin{equation}
I^{d} \;=\; (1-\lambda M)\odot I^{c} \;+\; (\lambda M)\odot \mathbf{c},
\end{equation}
where $\odot$ denotes element-wise multiplication, $\lambda \in [0,1]$ is the mask coefficient, and
$\mathbf{c} \in \mathbb{R}^{1 \times 1 \times 3}$, $\mathbf{c} \in [0,1]$ represents the chromatic aberration value.

\paragraph{Haze.}
Given a clean image $I^c \in \mathbb{R}^{H \times W \times 3}$, previous methods~\citep{li2019benchmarking}
often rely on the atmospheric scattering model (ASM) to generate a hazy image
$I^h \in \mathbb{R}^{H \times W \times 3}$ as
\begin{equation}
\begin{split}
I^{h} &= I^{c} \times T + \alpha \times (1-T), \\
T &= e^{-\beta \times d},
\end{split}
\end{equation}
where $\alpha \in \mathbb{R}^{3}$ denotes the atmospheric light,
$T \in \mathbb{R}^{H \times W \times 1}$ denotes the transmission map,
and $\beta \in \mathbb{R}^{1}$, $d \in \mathbb{R}^{H \times W \times 1}$ denote the haze density and depth map, respectively.

\begin{figure}[t!]
\centering
\includegraphics[width=\linewidth]{./appendix_img/promptir_finetune_curve.png}
\caption{
% \textcolor{red}{
Restoration performance versus the proportion of target-domain degradation patterns used for fine-tuning. Using PromptIR~\citep{potlapalli2023promptir} on WeatherBench~\cite{guan2025weatherbench}, performance improves steadily as more target-domain adaptive data is included.
%
%The result shows that DDTNet can enhance the restoration model even with a small amount of domain-adaptive pairs, while achieving further improvements as more pairs become available.
%fine-tuning data ratios on PromptIR~\citep{potlapalli2023promptir}. We employ DDTNet to transfer degradation patterns from WeatherBench~\cite{guan2025weatherbench} (target domain) images onto clean images, thereby synthesizing domain-adaptive training pairs. The numerical values indicate the percentage of the WeatherBench dataset sampled to generate these pairs. Specifically, '0' denotes the baseline model without domain-adaptive fine-tuning, while '100' corresponds to utilizing the entire WeatherBench dataset for data generation.
% }
}
\label{fig:Finetune_curve}
\vspace{-0.22in}
\end{figure}

% \textcolor{red}{
\section{Impact of Fine-Tuning Data Scale on Adaptation Performance}
Figure~\ref{fig:Finetune_curve} illustrates the restoration performance of PromptIR~\citep{potlapalli2023promptir} on the WeatherBench~\cite{guan2025weatherbench} dataset when fine-tuned with varying proportions of domain-adaptive pairs.
The baseline model ($0\%$) without any fine-tuning data achieves $21.20$ dB PSNR.
Using $10\%$ and $25\%$ of domain-adaptive pairs achieves $21.34$ dB and $21.57$ dB, yielding noticeable gains of $0.14$ dB and $0.37$ dB over the baseline.
The restoration performance steadily improves as more domain-adaptive pairs are used, reaching a best result of $21.97$ dB, which yields noticeable gains of $0.77$ dB compared to the baseline when the full set of domain-adaptive pairs is utilized.
These results demonstrate that DDTNet enhances the restoration model even with limited domain-adaptive data, while achieving further improvements as more pairs become available.
% }
%Figure~\ref{fig:Finetune_curve} illustrates the PSNR trend of the PromptIR model when fine-tuned on the WeatherBench~\cite{guan2025weatherbench} with varying data ratios. The baseline model without fine-tuning (0\%) starts at 21.20 dB. Incorporating just 10\% of the domain-adaptive data already yields an improvement to 21.34 dB. As the data ratio increases to 25\% and 50\%, the PSNR steadily rises to 21.57 dB and 21.63 dB, respectively. The performance continues to grow, reaching 21.75 dB at 75\% usage, and peaks at 21.97 dB (a total gain of 0.77 dB) when 100\% of the WeatherBench-generated data is utilized. These results confirm that DDTNet effectively bridges the domain gap, with the model consistently benefiting from the synthesized data at all scales.

%---------------------------------------------------------------
\section{Additional Qualitative Results}
\label{sec:app:qualitative}
%---------------------------------------------------------------

\begin{figure*}[t]
  \centering
  \includegraphics[
    width=\appfigwidth,
    height=0.9\textheight,
    keepaspectratio
  ]{appendix_img/appendix_transfer.pdf}
  \vspace{-0.4em}
  \caption{Qualitative results of degradation-transferred images.}
  \label{fig:app_trans}
  \vspace{-0.3em}
\end{figure*}

\begin{figure*}[t]
  \centering
  \includegraphics[
    width=\appfigwidth,
    height=0.9\textheight,
    keepaspectratio
  ]{appendix_img/appendix_promptir.pdf}
  \vspace{-0.4em}
  \caption{Qualitative comparison of PromptIR~\citep{potlapalli2023promptir} on WeatherStream~\citep{zhang2023weatherstream} (left) and WeatherBench~\citep{guan2025weatherbench} (right) between its baseline and DDTNet-enhanced versions.}
  \label{fig:app_promptir}
  \vspace{-0.3em}
\end{figure*}

\begin{figure*}[t]
  \centering
  \includegraphics[
    width=\appfigwidth,
    height=0.9\textheight,
    keepaspectratio
  ]{appendix_img/appendix_adair.pdf}
  \vspace{-0.4em}
  \caption{Qualitative comparison of AdaIR~\citep{cui2025adair} on WeatherStream~\citep{zhang2023weatherstream} (left) and WeatherBench~\citep{guan2025weatherbench} (right) between its baseline and DDTNet-enhanced versions.}
  \label{fig:app_adair}
  \vspace{-0.3em}
\end{figure*}

\begin{figure*}[t]
  \centering
  \includegraphics[
    width=\appfigwidth,
    height=0.9\textheight,
    keepaspectratio
  ]{appendix_img/appendix_dfpir.pdf}
  \vspace{-0.4em}
  \caption{Qualitative comparison of DFPIR~\citep{tian2025degradation} on WeatherStream~\citep{zhang2023weatherstream} (left) and WeatherBench~\citep{guan2025weatherbench} (right) between its baseline and DDTNet-enhanced versions.}
  \label{fig:app_dfpir}
  \vspace{-0.3em}
\end{figure*}

Figure~\ref{fig:app_trans} presents additional degradation-transferred results along with their corresponding degradation features.
These results demonstrate that DDTNet successfully disentangles and transfers degradation patterns, thereby producing realistic degradation-transferred images.
Figures~\ref{fig:app_promptir}--\ref{fig:app_dfpir} present additional restored images generated by PromptIR~\citep{potlapalli2023promptir}, AdaIR~\citep{cui2025adair}, and DFPIR~\citep{tian2025degradation}, respectively.
These results demonstrate that these methods effectively enhance the baseline model, removing artifacts and producing more realistic images.
